# Supplementary material for: Applications of the Octet Baryon Quark-Meson Coupling Model to Hybrid Stars
Source: arXiv:1001.4318 source file (2010-01-25)
Supplement: Supplementary file 1 [file AppendixC_misc.tex]

\chapter{Miscellaneous}\label{sec:misc}
